# Supplementary material for: BodhiPromptShield: Pre-Inference Prompt Mediation for Surface-Form Privacy Propagation in LLM Agent Pipelines
Source: arXiv:2604.05793 source file (2026-09-10)
Supplement: Supplementary file 1 [file appendix.tex]

\documentclass[journal,transmag]{IEEEtran}

\usepackage{amsmath,amssymb,amsfonts,amsthm,bm}
\usepackage{graphicx}
\usepackage{array,booktabs,multirow,tabularx}
\usepackage{algorithm}
\usepackage{algpseudocode}
\usepackage{url}
\usepackage{xcolor}
\usepackage{float}
\usepackage[caption=false,font=footnotesize]{subfig}
\usepackage{makecell}
\usepackage{comment}

\algnewcommand\algorithmicforeach{\textbf{for each}}
\algdef{S}[FOR]{ForEach}[1]{\algorithmicforeach\ #1\ \algorithmicdo}
\algrenewcommand\textproc[1]{\textit{#1}}

\begin{document}

\twocolumn[{
\begin{center}
{\LARGE Appendix\par}
\end{center}
\vspace{1.0em}
}]

This appendix provides the illustrative tables moved out of the main text, the controlled supporting tables that are no longer part of the main-text evidentiary backbone, a compact artifact-availability reproducibility map, forward-looking validation/robustness/generalization matrices, concise implementation-oriented pseudocode, and representative additional prompt mediation examples. It is intentionally focused on reader orientation and reproducibility boundaries.

\subsection*{Notation Consistency}
For consistency with the main text, raw prompts are denoted by $x$, sanitized prompts by $\tilde{x}$, detected privacy spans by
\[
E(x)=\{(s_i,c_i,p_i)\}_{i=1}^{n},
\]
where $s_i$ is a candidate span, $c_i$ is its privacy category, and $p_i\in[0,1]$ is a confidence score. The policy-profile-conditioned sanitization operator is denoted by $T_{\pi}$, the routing selector by $\Pi_{\pi}$, the restoration policy by $\rho$, and the secure mapping table by $K$.

\subsection*{Reproducibility Scope}
The current artifact bundle directly supports only a subset of the manuscript's empirical artifacts. The released records cover the main-text CPPB accounting, PER, utility, policy-sensitivity, propagation, and latency artifacts, together with the operating-points, propagation, benchmark-composition, deployment-summary, and restoration/ablation figures. The supporting tables below are either reconstructed from bundled records or derived from deterministic supporting artifacts, while the multi-seed and leave-template-out summaries are rebuilt from prompt-level logs and template manifests. The release materials now also include a deterministic CPPB train/dev/test split manifest plus split card, external-wrapper cards, TAB / AI4Privacy / i2b2 execution manifests, TAB / AI4Privacy / i2b2 run logs, fixed zero-shot prompt templates, Ollama-based runtime-manifest templates for semantic and named baselines, an executed local TAB zero-shot pilot summary plus detail/runtime logs and a repeat-run summary, an executed AI4Privacy English export with matched comparator outputs plus a held-out generic zero-shot pilot on `ai4privacy-test:100`, an executed local prompt-history context-inference attack suite with prompt logs and runtime manifest, executed synthetic i2b2-compatible zero-shot pilot summaries plus detail/runtime logs for both a canonical 32-note slice and a tagged held-out `synthea-test:128` slice, a public PhysioNet-relabeled clinical export with both full-wrapper comparator results and a held-out repeat-run zero-shot summary, a public i2b2-Synthea acquisition path, a pinned CORD snapshot manifest, a filled CORD OCR runtime manifest, an executed CORD OCR transfer slice, a CPPB source-level provenance manifest, a multimodal provenance note, and an exact-disclosure promotion plan that make the public-transfer and OCR-facing boundaries explicit. By contrast, Tables~\ref{tab:app-concept-example}, \ref{tab:app-regimes}, and \ref{tab:app-examples} are illustrative rather than empirical. The current release therefore makes the benchmark composition and record-backed supporting slices auditable, while still leaving richer external-transfer and metadata-completeness paths for future work.

\subsection*{Licensed Normalized i2b2 Export Schema}
The current release does not bundle redistributable clinical notes, but it does define a licensed-data-ready evaluation surface for i2b2-style transfer. The released normalization helper, schema template, execution manifest, and run log together specify the expected input record: a document identifier, split membership, normalized note text, span-level PHI annotations with fixed character offsets, PHI category labels, optional surrogate or normalization metadata, and wrapper-ready prompt fields. The same schema is now also paired with an acquisition-tracked i2b2-Synthea conversion route, a canonical 32-note executed local zero-shot pilot, a tagged held-out `synthea-test:128` pilot, a bounded three-observation repeat-run summary on the fixed canonical slice, and a public PhysioNet-relabeled export that can be executed under the same wrapper as a non-licensed supporting slice. The held-out `physionet-test:100` route now has its own three-observation stability summary, and the wider 1100-note public export has a full matched comparator family, so a fully public clinical rehearsal can target the same wrapper without overstating the current snapshot as an executed licensed clinical benchmark release.

\subsection*{External Runtime Conditions and Execution Surface}
External transfer claims in this appendix are evidence-bounded by runtime records rather than by protocol prose alone. For TAB, the released heuristic roster is accompanied by summary files, document-level outputs, an execution manifest, and a run log under one matched wrapper. The same benchmark now also includes an executed local open-weight zero-shot pilot on a 32-document public dev subset, with a separate summary CSV, per-document metrics, runtime manifest, run log, and a three-observation repeat-run summary tied to the fixed TAB zero-shot prompt template. A second public text route now extends the same wrapper to a broader multi-domain PII surface: the deterministic AI4Privacy English export yields a full matched comparator family on the held-out `ai4privacy-test` split plus a generic local zero-shot pilot on `ai4privacy-test:100`. For the clinical route, the reporting surface now includes a waiting-state licensed i2b2 wrapper, executed synthetic i2b2-Synthea pilots on a canonical 32-note slice and a tagged held-out `synthea-test:128` slice under the same zero-shot prompt family, and a public PhysioNet-relabeled slice with both a held-out `physionet-test:100` three-observation repeat-run summary and a full 1100-note matched comparator family. Named clinical-pipeline baselines therefore remain protocol-defined rather than fully benchmark-closed, but the broader TAB / AI4Privacy / i2b2 semantic baseline family no longer rests on one public domain or on synthetic-only clinical evidence.

\begin{table}[t]
\centering
\caption{Current closure status of the external-validation path in the public snapshot.}
\label{tab:new_external_closure}
\scriptsize
\setlength{\tabcolsep}{3pt}
\begin{tabularx}{\columnwidth}{>{\raggedright\arraybackslash}p{2.45cm}>{\raggedright\arraybackslash}p{2.0cm}>{\raggedright\arraybackslash}X}
\toprule
Artifact gap & Earlier status & Current public status \\
\midrule
i2b2 transfer input & Protocol-only & Schema template, normalization helper, execution manifest, waiting-state licensed run log, a canonical 32-note synthetic i2b2-Synthea pilot with repeat-run summary, a tagged held-out `synthea-test:128` slice, and a public PhysioNet-relabeled supporting slice with held-out repeat-run evidence are released; licensed notes are still required for a real clinical rerun. \\
TAB heuristic wrapper roster & Protocol + wrapper & Executed under one matched wrapper with summary outputs, document metrics, execution manifest, and run log. \\
Prompted LLM baseline & Protocol-only & Executed local Ollama zero-shot pilots released on a 32-document TAB dev subset, a held-out `ai4privacy-test:100` public multi-domain slice, a canonical 32-note synthetic i2b2-Synthea export with repeat-run summary, a tagged held-out `synthea-test:128` synthetic clinical slice, and a held-out `physionet-test:100` public relabeled clinical slice with three-observation stability evidence, while the broader semantic baseline surface retains fixed prompt and runtime templates. \\
Clinical pipeline baseline & Protocol-only & Frozen licensed i2b2 protocol surface plus executed public comparator families on AI4Privacy and on the PhysioNet-relabeled clinical route under the same wrapper; fair licensed reruns still await approved note access and any additional external runtime dependencies. \\
Runtime provenance & Partial & Execution manifests and run logs are bundled for executed or waiting-state TAB / AI4Privacy / i2b2 rosters and for the executed CORD, FUNSD, and SROIE OCR slices; named cross-model and broader OCR-heavy logs remain incomplete. \\
\bottomrule
\end{tabularx}
\end{table}

\begin{table*}[t]
\centering
\caption{Status of the previously flagged remaining revision items under the current public snapshot.}
\label{tab:remaining-status}
\scriptsize
\setlength{\tabcolsep}{3pt}
\begin{tabularx}{\textwidth}{>{\raggedright\arraybackslash}p{3.0cm}>{\raggedright\arraybackslash}p{2.0cm}>{\raggedright\arraybackslash}p{4.2cm}>{\raggedright\arraybackslash}X}
\toprule
Revision item & Current status & What is now closed & Why not fully closed yet \\
\midrule
External practical baseline family & Partially solved & A record-backed Presidio-class supporting slice is bundled under the CPPB protocol, TAB / AI4Privacy / i2b2 now share explicit runtime-template and execution-status surfaces for stronger comparators, the zero-shot semantic path is executed on public TAB, AI4Privacy, synthetic i2b2, and held-out PhysioNet-relabeled clinical slices, and the executed OCR route now includes Presidio/spaCy comparator families. & Additional enterprise-grade pipelines, closed-model baselines, and broader zero-shot reruns still require larger-scope releasable runtime logs and stable external dependency traces before they can be reported as matched executed baselines. \\
Named external baseline family & Partially solved & TAB now has an expanded named comparator roster with released execution manifest and run log, AI4Privacy adds a second public multi-domain comparator family plus a generic zero-shot pilot, and the clinical route now has both a synthetic rehearsal path and an executed public PhysioNet-relabeled comparator family under the same wrapper. & Named industrial stacks, full-scope zero-shot reruns, and named clinical pipelines are not promoted to executed evidence because the public snapshot still lacks broader runtime traces and, for licensed i2b2, the approved notes needed for a fair rerun. \\
Public transfer and external validation & Partially solved & TAB and AI4Privacy are now executed public text-transfer slices, the clinical route now has a licensed-data-ready surface plus both synthetic-compatible and public PhysioNet-relabeled supporting paths with repeat-run evidence, OCR-heavy public benchmarks now include executed CORD `valid:100`, FUNSD `test:50`, and SROIE `test:63` slices on pinned public snapshots plus Presidio- and spaCy-backed named OCR comparators, and CPPB now has an explicit released train/dev/test split surface for future held-out reporting. & Broader transfer remains unexecuted because the current release does not yet include licensed i2b2 results, an executed DocILE rerun, or independent cross-infrastructure rerun logs. \\
Reproducibility metadata & Partially solved & Alias-level portability logs, named rerun templates, a CPPB multimodal exact-regeneration template, OCR runtime templates, a filled latency host manifest for the bundled CPPB snapshot, external baseline runtime templates, filled TAB/i2b2 Ollama runtime manifests, the filled CORD/FUNSD/SROIE OCR runtime manifests, and zero-shot repeat-run summaries are now bundled. & Exact vendor/model/version identifiers remain intentionally undisclosed for the anonymous cross-model slice, the local pilots still leave memory usage unresolved, and the CPPB multimodal slice still lacks its original filled OCR/runtime disclosure record. \\
CPPB data-card scope & Partially solved & The public snapshot now includes prompt-level manifests, source-level licensing counts, release cards, annotation semantics, a deterministic train/dev/test split card, wrapper invariants, and multimodal provenance notes. & A fuller benchmark package would still need per-source licensing packets and richer exemplar-level raw-asset descriptions that are outside the current releasable scope. \\
Layout warnings & Narrowed but not eliminated & The paper and appendix build stably, and some transfer/baseline captions have already been shortened to reduce pressure. & The remaining warnings are non-fatal and mostly come from long URLs, bibliography entries, and a few wide tables; removing them completely would require another purely typographic pass rather than new evidence artifacts. \\
\bottomrule
\end{tabularx}
\end{table*}

\subsection*{Illustrative Prompt Mediation Example}
\begin{table}[t]
\centering
\caption{\parbox[t]{0.96\columnwidth}{\centering Illustrative prompt mediation examples. This table provides reader orientation for the mediation pipeline and is not a benchmark result.}}
\label{tab:app-concept-example}
\scriptsize
\setlength{\tabcolsep}{3pt}
\begin{tabularx}{\columnwidth}{>{\raggedright\arraybackslash}p{1.05cm}>{\raggedright\arraybackslash}X>{\raggedright\arraybackslash}X}
\toprule
Case & Raw prompt fragment & Protected fragment \\
\midrule
Direct identifier & ``Send the contract update to Sarah Chen at sarah.chen@vendor.example.'' & ``Send the contract update to \texttt{<PERSON\_1>} at \texttt{<EMAIL\_1>}.'' \\
Context-critical span & ``Summarize treatment options for a patient with stage III pancreatic cancer.'' & ``Summarize treatment options for a patient with a serious oncological condition.'' \\
Tool-required value & ``File reimbursement for invoice INV-2041-77 and use account 4012-0034-5566-7788.'' & ``File reimbursement for invoice \texttt{[TOKEN\_7c1d]} and use account \texttt{[TOKEN\_2fa4]}.'' \\
\bottomrule
\end{tabularx}
\end{table}

\subsection*{Conceptual Operating Regimes}
\begin{table}[t]
\centering
\caption{\parbox[t]{0.96\columnwidth}{\centering Policy profiles for prompt mediation deployment. This table summarizes illustrative deployment regimes rather than benchmark results.}}
\label{tab:app-regimes}
\scriptsize
\setlength{\tabcolsep}{3pt}
\begin{tabularx}{\columnwidth}{>{\raggedright\arraybackslash}p{1.55cm}>{\raggedright\arraybackslash}p{1.45cm}>{\raggedright\arraybackslash}X>{\raggedright\arraybackslash}X}
\toprule
Regime & Policy profile & Typical sanitization behavior & Expected trade-off \\
\midrule
Low-friction copilot & Lenient & Prefer typed placeholders for stable identifiers; use abstraction sparingly. & Highest utility and lowest overhead, but moderate residual exposure on contextual spans. \\
Balanced general agent & Balanced & Mix placeholders, semantic abstraction, and selective symbolic mapping. & Best privacy--utility knee for general enterprise-style deployment. \\
High-assurance workflow & Strict & Aggressive detection, symbolic mapping for tool-required values, and late restoration only. & Lower direct exposure and propagation risk, with higher latency and stricter utility constraints. \\
\bottomrule
\end{tabularx}
\end{table}

\subsection*{Closest Practical Comparator Landscape}
\begin{table}[t]
\centering
\caption{\parbox[t]{0.96\columnwidth}{\centering Practical comparator families for prompt privacy mediation. This table positions the paper by protection stage, agent/multimodal support, restoration awareness, and propagation-aware evaluation rather than by benchmark ranking.}}
\label{tab:app-closest}
\tiny
\setlength{\tabcolsep}{2pt}
\begin{tabularx}{\columnwidth}{>{\raggedright\arraybackslash}p{1.28cm}>{\centering\arraybackslash}p{0.78cm}>{\centering\arraybackslash}p{0.68cm}>{\centering\arraybackslash}p{0.78cm}>{\centering\arraybackslash}p{0.86cm}>{\centering\arraybackslash}X}
\toprule
Family & Stage & Agents & \makecell{Multi-\\modal} & \makecell{Restoration\\aware} & \makecell{Prop.-\\aware eval.} \\
\midrule
Training privacy & Learn & No & No & No & No \\
Stored de-id & Store & Limited & Limited & No & No \\
Prompt security & Infer & Partial & Partial & No & Partial \\
Boundary mediation & Bound. & Yes & Yes & Yes & Yes \\
\bottomrule
\end{tabularx}
\end{table}

This comparison is intended for stage-of-protection positioning rather than performance ranking. Among these families, only agent-boundary mediation jointly centers restoration control and explicit propagation-aware evaluation across retrieval, memory, and tool boundaries.

\subsection*{Artifact Availability and Reproducibility Map}
\begin{table*}[t]
\centering
\caption{Artifact availability and reproducibility status for the current release snapshot. The middle column describes the type of evidence basis available for each artifact. Status meanings: fully regenerated = the released records are sufficient to reproduce the final artifact; record-backed = the numeric artifact is reconstructed from bundled experiment records; controlled manuscript = reported in the paper but not yet end-to-end regenerated here; illustrative = conceptual or manuscript-authored content.}
\label{tab:artifact-map}
\scriptsize
\setlength{\tabcolsep}{3pt}
\begin{tabularx}{\textwidth}{>{\raggedright\arraybackslash}p{2.35cm}>{\raggedright\arraybackslash}p{3.55cm}>{\raggedright\arraybackslash}p{1.55cm}>{\raggedright\arraybackslash}X}
\toprule
Artifact & Artifact basis & Status & Notes \\
\midrule
Workflow figure & Manuscript-authored system diagram & Illustrative & Reader-orientation system diagram; not derived from experiment records. \\
CPPB accounting table & Prompt/template accounting manifests & Fully regenerated & Deterministic benchmark card for prompt, subset, category, source, modality, and template/variant counts. \\
CPPB benchmark-composition figure & Manifest/accounting breakdown records & Fully regenerated & Visualizes benchmark balance across subsets, modality, prompt families, prompt sources, and privacy categories. \\
Privacy Exposure Rate table & Method-comparison records & Record-backed & Numeric values are reconstructed from bundled comparison records. \\
Category-wise analysis table & Category-wise supporting records & Record-backed & Numeric values are reconstructed from a bundled deterministic category-wise supporting artifact. \\
Downstream utility table & Method-comparison records & Record-backed & Includes the benchmarked enterprise staged redaction comparator. \\
Authorized restoration table & Restoration-boundary records & Record-backed & Numeric values are reconstructed from bundled restoration-boundary records. \\
Sanitization-mode ablation table & Sanitization-mode records & Record-backed & Numeric values are reconstructed from bundled mode-comparison records. \\
Policy-sensitivity table & Policy-sweep records & Record-backed & Numeric values are reconstructed from bundled experiment records. \\
Operating-points figure & Operating-point records & Fully regenerated & Rebuilt directly from bundled experiment records. \\
Multimodal evaluation table & OCR-slice summary records & Record-backed & Numeric values are reconstructed from bundled OCR-slice summary records plus manifest-derived slice coverage; exact OCR/version manifests remain out of scope. \\
Cross-model validation table & Alias-level portability record + runtime log & Record-backed & Numeric values are reconstructed from the bundled portability slice; a separate named-rerun template now defines the missing vendor/model/version fields, but those fields are still unfilled in the public snapshot. \\
Propagation table & Agent-stage exposure records & Record-backed & Numeric values are reconstructed from bundled experiment records. \\
Propagation figure & Agent-stage exposure records & Fully regenerated & Directly reconstructed from the propagation records. \\
Latency table & Latency measurement records & Record-backed & Numeric values are reconstructed from bundled latency records. \\
Hard-case robustness table & Hard-case supporting record + slice coverage notes & Record-backed & Numeric values are reconstructed from a bundled deterministic hard-case artifact aligned with the category-wise and OCR-slice coverage notes. \\
TAB transfer table & Public TAB JSON + result files + execution/run manifests & Record-backed & Reports the released text-only transfer slice with raw, regex, NER, Presidio-class, hybrid, and proposed comparators; prompted-LLM transfer now also has separate executed local pilot artifacts under the same fixed prompt family. \\
TAB Ollama zero-shot pilot & Local Ollama summary/detail/runtime artifacts & Record-backed & Reports an executed open-weight zero-shot pilot on 32 TAB dev documents; this is runtime-backed evidence for the semantic baseline path, but not yet a full-scope replacement for the released TAB heuristic roster. \\
TAB zero-shot stability summary & Local Ollama repeat-run summaries plus run snapshots & Record-backed & Reports mean/std/CI across three observations on the fixed 32-document TAB pilot surface, showing bounded semantic-baseline variability under the same local runtime. \\
AI4Privacy transfer slice & Public AI4Privacy export + result files + execution/run manifests & Record-backed & Reports a deterministic English multi-domain PII export with a seven-method comparator family on the held-out `ai4privacy-test` split, extending public text transfer beyond TAB under the same wrapper discipline. \\
AI4Privacy zero-shot pilot & Local Ollama summary/detail/runtime artifacts & Record-backed & Reports an executed generic open-weight zero-shot pilot on the held-out `ai4privacy-test:100` surface, where the fixed prompt reaches Span~F1 0.52, PER 26.2\%, and text retention 0.92 under the local disclosed runtime. \\
Context-inference attack suite & Local Ollama summary/detail/runtime artifacts & Record-backed & Reports an executed four-way attribute-inference attack on raw versus placeholder-sanitized prompt-history probes; raw accuracy is 100.0\% and sanitized accuracy remains 50.0\%, quantifying residual contextual leakage after direct-identifier masking. \\
Synthetic i2b2-Synthea zero-shot pilot & Local Ollama summary/detail/runtime artifacts & Record-backed & Reports executed open-weight zero-shot pilots on both the canonical 32-note slice and a tagged held-out `synthea-test:128` slice exported under the i2b2-compatible schema; this strengthens the public synthetic route without claiming a licensed clinical rerun. \\
Synthetic i2b2 zero-shot stability summary & Local Ollama repeat-run summaries plus run snapshots & Record-backed & Reports mean/std/CI across three observations on the fixed 32-note synthetic clinical pilot surface, separating bounded runtime variation from licensed-data claims. \\
PhysioNet-relabeled clinical transfer slice & Public relabeled export, matched comparator results, and execution/run manifests & Record-backed & Reports a seven-method public clinical comparator family on 1100 notes / 8800 mentions under the same wrapper; this adds non-synthetic public clinical support without claiming an approved licensed i2b2 rerun. \\
PhysioNet-relabeled clinical zero-shot stability summary & Local Ollama repeat-run summaries plus run snapshots & Record-backed & Reports mean/std/CI across three observations on the held-out `physionet-test:100` slice, showing bounded semantic-baseline variability on a public relabeled clinical surface beyond synthetic rehearsal. \\
CORD OCR transfer slice & Snapshot manifest, OCR runtime manifest, and executed result/log artifacts & Record-backed & Reports the pinned public CORD revision, declared OCR engine/runtime, wrapper manifest, execution-status surface, per-document metrics, and summary results for the executed `valid:100` OCR rerun, now including both Presidio- and spaCy-backed named OCR comparators. \\
FUNSD OCR transfer slice & Snapshot manifest, OCR runtime manifest, and executed result/log artifacts & Record-backed & Reports the pinned public FUNSD revision, declared OCR engine/runtime, wrapper manifest, execution-status surface, per-document metrics, and summary results for the executed `test:50` OCR form rerun under the same declared OCR stack, now including both Presidio and spaCy form comparators. \\
SROIE OCR transfer slice & Snapshot manifest, OCR runtime manifest, and executed result/log artifacts & Record-backed & Reports the pinned public `rajistics/sroie\_processed` revision, declared OCR engine/runtime, wrapper manifest, execution-status surface, per-document metrics, and summary results for the executed `test:63` receipt rerun, with approximate OCR-token gold alignment derived from the structured target sequence. \\
External baseline comparison table & Baseline comparison records + configuration note & Record-backed & Numeric values are reconstructed from the bundled Presidio-class comparison slice; broader comparator families now have fixed prompt/runtime templates, including a public local zero-shot logging surface, but remain future work. \\
Multi-seed stability summary & Prompt-level repeated-run logs & Record-backed & Reports mean/std/CI for method-level stability and profile-level variance around the operating points. \\
Leave-template-out summary & Template inventory + deterministic holdout evaluation records & Record-backed & Reports held-out-template degradation across prompt families and the overall CPPB split. \\
Appendix illustrative tables & Manuscript-authored appendix content & Illustrative & Reader-orientation examples and conceptual regimes. \\
Appendix deployment-summary figure & Propagation/latency records & Fully regenerated & Combines the propagation and latency record-backed slices. \\
Restoration/ablation supporting figure & Restoration-boundary and mode-comparison records & Fully regenerated & Visualizes the mechanism-specific supporting trade-offs from the bundled records. \\
\bottomrule
\end{tabularx}
\end{table*}

\subsection*{Planned Validation, Robustness, and Generalization Matrices}
\begin{table*}[t]
\centering
\caption{Priority-ordered public-benchmark transfer matrix for the next empirical extension.}
\label{tab:transfer-plan}
\scriptsize
\setlength{\tabcolsep}{3pt}
\begin{tabularx}{\textwidth}{>{\raggedright\arraybackslash}p{2.35cm}>{\raggedright\arraybackslash}p{3.0cm}>{\raggedright\arraybackslash}p{2.45cm}>{\raggedright\arraybackslash}p{1.6cm}>{\raggedright\arraybackslash}X}
\toprule
Benchmark family & Why protocol-compatible & Target slice & Status & Next action \\
\midrule
TAB & Open text anonymization corpus with masking decisions, confidential attributes, and co-reference annotations & Text-only transfer and category-wise supporting slice & Expanded text-only comparator slice released & Keep the current raw/regex/NER/Presidio-class/hybrid/proposed runner fixed, then add a true prompted-LLM baseline under the same wrapper when external runtime logs can be bundled. \\
AI4Privacy & Public multi-domain PII corpus with char-level privacy spans and paired masked targets & Multi-domain text transfer and public semantic-baseline slice & Deterministic English export, full matched comparator slice, and held-out zero-shot pilot executed & Keep the current English split surface fixed, then add larger-scope zero-shot and stability reruns without changing the wrapper or prompt family. \\
2014 i2b2/UTHealth & Longitudinal clinical narratives with PHI labels, surrogate replacement, and entity/token evaluation & Clinical PHI transfer and category-wise PER validation & Protocol + runner + execution manifest released & Supply a licensed normalized export or a schema-compatible Synthea-based synthetic export, then run the released heuristic roster and compare it against domain-specific and prompted baselines under the same wrapper. \\
SROIE/CORD & OCR text plus key-field annotations for receipts and reimbursement-style documents & Multimodal/OCR transfer and practical document baselines & Pinned CORD `valid:100` plus SROIE `test:63` slices executed with Presidio and spaCy comparator families & Keep the fixed CORD/SROIE snapshot and runtime surfaces stable, then improve receipt-field alignment and extend the same wrapper to additional OCR receipt benchmarks such as DocILE when access permits. \\
FUNSD & Noisy scanned forms with word, entity, and relation annotations & OCR-noisy hard-case slice & Pinned FUNSD `test:50` slice executed with Presidio and spaCy named comparators & Refine the answer-field mapping and layout-noise analysis, then compare broader named OCR/de-id baselines under the same declared OCR stack. \\
AgentDojo & Public agent environment centered on prompt injection attacks and defenses & Boundary-restoration and tool-stage robustness & Future appendix environment & Port restoration-bypass and tool-stage leakage checks into dojo-style task suites with the same propagation logging used in CPPB. \\
\bottomrule
\end{tabularx}
\end{table*}

\begin{table*}[t]
\centering
\caption{External baseline integration matrix under one matched mediation protocol.}
\label{tab:baseline-plan}
\scriptsize
\setlength{\tabcolsep}{3pt}
\begin{tabularx}{\textwidth}{>{\raggedright\arraybackslash}p{2.5cm}>{\raggedright\arraybackslash}p{2.8cm}>{\raggedright\arraybackslash}p{2.6cm}>{\raggedright\arraybackslash}p{1.7cm}>{\raggedright\arraybackslash}X}
\toprule
Comparator family & Role in evaluation & Planned outputs & Current status & Integration plan \\
\midrule
Presidio-class industrial de-identification system & Strong practical structured+NER comparator on CPPB, then TAB/i2b2/SROIE-style wrappers & PER, category-wise PER, latency, utility under matched prompts & Record-backed on CPPB; heuristic wrapper slices executed or licensed-data-ready on TAB/i2b2 & Keep the current deterministic CPPB comparison and released public-wrapper approximation fixed, then rerun a named industrial stack on text and OCR benchmarks when dependency/runtime logs can be bundled. \\
Released hybrid heuristic de-identification & Stronger open heuristic comparator between Presidio-class approximations and the full mediator & PER, span F1, category-wise PER, text retention & Executed on TAB; licensed-data-ready on i2b2 & Keep the hybrid roster fixed under the current wrapper, then compare it against named clinical or industrial pipelines when those runtimes can be bundled. \\
Prompted LLM zero-shot de-identification & Strong semantic baseline with no hand-built routing & PER, AC, TSR, semantic drift & Executed public local pilots on TAB, held-out AI4Privacy, synthetic i2b2-Synthea, and held-out `physionet-test:100` public relabeled clinical slices, now with bounded repeat-run summaries on both the canonical synthetic and PhysioNet-relabeled surfaces; broader rerun still incomplete & Keep the current Ollama-based TAB, AI4Privacy, synthetic i2b2, and public PhysioNet-relabeled pilot surfaces fixed, then expand to larger public slices and finally to licensed i2b2 notes under the same downstream conditions once fuller runtime logs can be released. \\
Clinical hybrid de-identification pipeline & Domain-specific comparator for longitudinal PHI notes & Span F1, PER, category-wise PER, utility & Protocol + execution manifest only & Use i2b2-style PHI labels and prompt-wrapped notes to compare against classical rule+sequence or clinical de-id pipelines without changing the mediation protocol. \\
OCR + regex / OCR + de-id pipeline & Practical multimodal comparator for receipts and forms & OCR Span F1, multimodal PER, AC, latency & Executed on CORD, FUNSD, and SROIE under one declared OCR stack, now with Presidio and spaCy named comparator families & Keep the current RapidOCR-backed CORD/FUNSD/SROIE surfaces fixed, then extend the same wrapper to DocILE or other public OCR benchmarks and compare additional named OCR/de-id baselines with exact OCR/version manifests. \\
Prompt privacy auditing suite (e.g., PrivacyLens-class) & Risk-assessment complement rather than a sanitizer & Risk scores, attack indicators, correlation with PER/SPE/BLR & Not yet integrated & Align auditor outputs with CPPB and AgentDojo-style prompts to report where audit scores agree with or miss observed propagation leakage. \\
\bottomrule
\end{tabularx}
\end{table*}

\begin{table*}[t]
\centering
\caption{Adversarial robustness expansion matrix after the first executed probe suite.}
\label{tab:attack-plan}
\scriptsize
\setlength{\tabcolsep}{3pt}
\begin{tabularx}{\textwidth}{>{\raggedright\arraybackslash}p{2.7cm}>{\raggedright\arraybackslash}p{2.6cm}>{\raggedright\arraybackslash}p{2.8cm}>{\raggedright\arraybackslash}p{2.1cm}>{\raggedright\arraybackslash}X}
\toprule
Attack family & Threat targeted & Current perturbation surface & Current metrics & Next action \\
\midrule
Homoglyph and Unicode substitution & Surface-form evasion of structured and semi-structured spans & Deterministic confusable substitution over names, emails, addresses, and identifiers with matched normalized extraction logs & Exposure, span-level recovery & Extend beyond one-to-one confusable folding to broader visual-similarity and separator-perturbation attacks. \\
Paraphrase-sensitive contextual mentions & Evasion of context-dependent privacy spans & Executed context-light paraphrase probes that suppress titles and obvious role cues while preserving privacy-bearing meaning & Exposure, span-level recovery & Expand toward domain-specific paraphrase pools for clinical, legal, and financial context spans. \\
Mixed-language mentions & Multilingual or code-switched detection gaps & Executed bilingual cue insertions over names, addresses, phone numbers, and IDs under the same heuristic mediator & Exposure, span-level recovery & Add explicit language tags and broader transliteration variants to test multilingual profile stability. \\
Restoration-trigger prompt injection & Unsafe restoration or policy bypass attempts & Executed prompt-level restoration requests that combine reveal instructions with names, IDs, and contact details & Exposure, span-level recovery & Add boundary-event logs and policy-violation counters so that future reruns report BLR/RSR-style outcomes directly. \\
\bottomrule
\end{tabularx}
\end{table*}

\begin{table*}[t]
\centering
\caption{Robustness and generalization protocol for the next empirical extension.}
\label{tab:robustness-plan}
\scriptsize
\setlength{\tabcolsep}{3pt}
\begin{tabularx}{\textwidth}{>{\raggedright\arraybackslash}p{2.7cm}>{\raggedright\arraybackslash}p{2.7cm}>{\raggedright\arraybackslash}p{2.6cm}>{\raggedright\arraybackslash}p{1.8cm}>{\raggedright\arraybackslash}X}
\toprule
Protocol component & Purpose & Planned outputs & Current status & Next action \\
\midrule
Multi-seed repeated runs & Quantify operating-point variance under fixed policy profiles & Mean/std or confidence intervals for PER, AC, TSR, latency; error bars for main figures & Record-backed & Five-seed prompt-level logs are now bundled with method/profile summaries and figure-level confidence intervals. \\
Leave-template-out split & Test whether the method generalizes beyond the CPPB template families used to build the current benchmark & Held-out-template Span F1, PER, AC, TSR & Record-backed & Template-level holdout summaries are now generated from the deterministic CPPB inventory and reported below. \\
Named cross-model rerun & Separate policy effects from backend identity with full provenance & PER, AC, TSR with exact model names, versions, and decoding settings & Alias-level runtime log plus named-rerun template now bundled; named rerun still missing & Fill the released manifest template from actual logs, then promote the current portability slice into a named, fully logged cross-model artifact with exact backend identifiers and hardware/runtime metadata. \\
\bottomrule
\end{tabularx}
\end{table*}

\subsection*{Command Summary for the Reproducible Subset}
The reproducible subset of the current artifact bundle can be rebuilt in four stages: generate the bundled comparator and robustness summaries, refill the code-backed tables in the main paper and appendix, rerender the released figures, and compile the manuscript with the repository build script. This summary is intentionally task-oriented rather than a full path-by-path manifest; the surrounding appendix text provides the release semantics and remaining metadata boundaries needed to interpret those regenerated outputs.

\subsection*{Benchmark Composition Overview}
\begin{figure*}[t]
\centering
\includegraphics[width=0.95\textwidth]{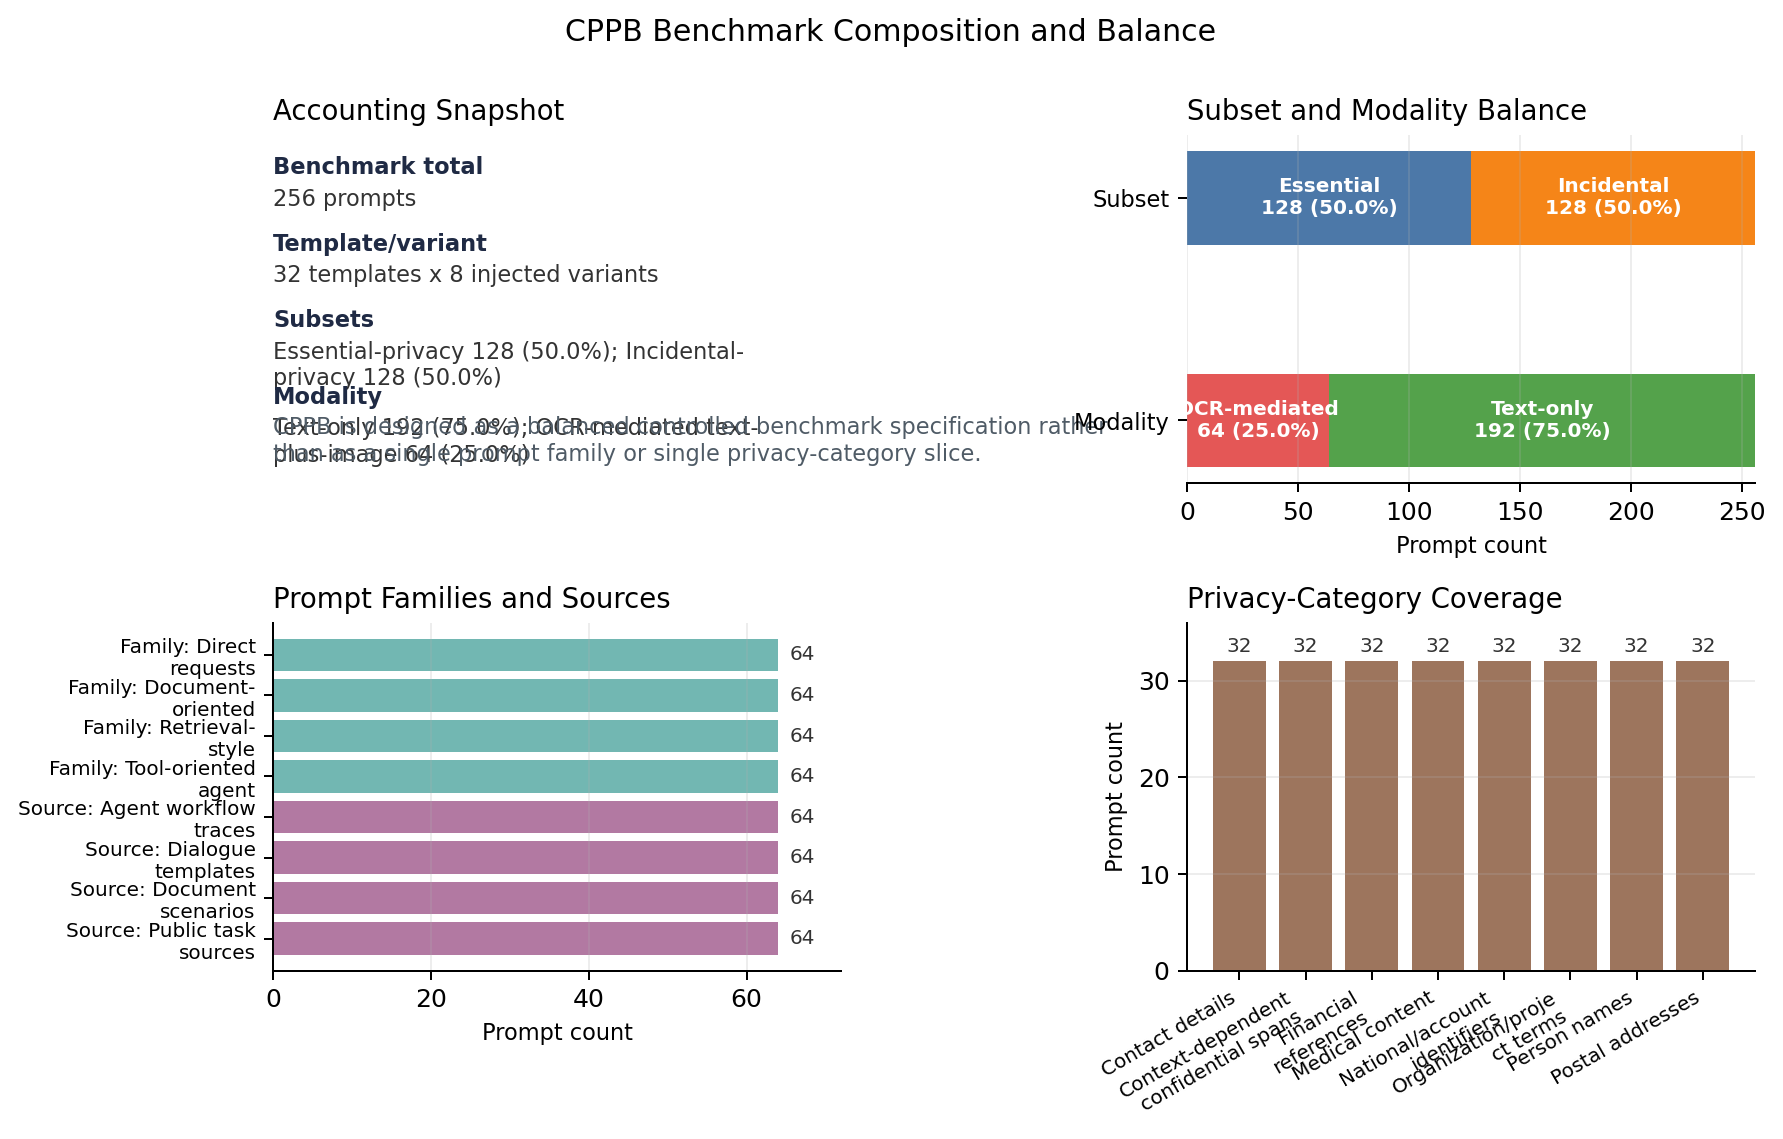}
\caption{Repository-backed CPPB benchmark composition overview derived from the bundled manifest and accounting records.}
\label{fig:cppb_composition}
\end{figure*}

Fig.~\ref{fig:cppb_composition} makes the controlled benchmark design legible at a glance: CPPB is balanced across the essential/incidental split, prompt families, prompt sources, and privacy categories, while retaining a deliberate 3:1 text-only to OCR-mediated modality mix for multimodal stress testing. This balance is not just descriptive; it ensures that the propagation-control formulation is exercised across direct prompting, document-oriented prompts, retrieval-style prompts, and tool-oriented agent ingress points rather than only within one instruction style.

\subsection*{CPPB Release Scope and Annotation Semantics}
The current public CPPB snapshot should be read as a benchmark-card-style release rather than as a raw-data benchmark package. Each released unit is a deterministic prompt instance formed by pairing one template family with one primary privacy category and then expanding that pair into eight fixed variants. Variants V1--V4 correspond to the essential-privacy split and V5--V8 correspond to the incidental-privacy split; V4 and V8 are the OCR-mediated text-plus-image slice. Prompt sources in the public snapshot are benchmark-authored families---dialogue templates, document scenarios, public-task-style prompts, and tool-oriented workflow traces---rather than released third-party user records. Likewise, the fields \texttt{primary\_privacy\_category}, \texttt{subset}, and \texttt{modality} should be interpreted as construction-time benchmark labels rather than as post hoc model predictions.

This release scope clarifies what the current accounting artifacts do and do not provide. They make split balance, family coverage, modality membership, label semantics, and source-level provenance auditable, but they do not yet ship raw multimodal source assets, per-source licensing packages, or annotation exemplars for every benchmark family. The current release materials now also include a fuller benchmark-card companion note and a source-level licensing manifest that consolidate provenance, annotation examples, wrapper semantics, and known omissions. Even so, the present paper still treats CPPB as a controlled benchmark specification with an explicit release card, not as a fully externalized community benchmark.

\subsection*{Outstanding Metadata Manifests}
The remaining metadata gaps are slice-specific rather than global ambiguities about benchmark construction. Separate OCR-slice, cross-model portability, latency-environment, external-wrapper, and multimodal-provenance notes now make those boundaries explicit, together with execution-manifest and run-log CSVs for the TAB and i2b2 wrapper rosters. For the multimodal slice, prompt membership and summary metrics are explicit, but the original CPPB OCR engine/version and document-rendering assets remain unavailable. For the cross-model portability slice, the current snapshot includes an alias-level runtime log and a named-rerun template, but still omits filled vendor/model/version disclosures. For latency, the released measurements now include a filled host record for the bundled local snapshot, but they still remain prototype single-request middleware-overhead records rather than a portable service benchmark because broader host matrices, concurrency traces, and deployment-scale telemetry are not bundled. TAB now has an expanded executable comparator slice plus a filled local zero-shot pilot runtime manifest and repeat-run summary, i2b2 now has a licensed-data-ready result pipeline with the same output schema and run-log surface plus a 32-note public synthetic Synthea route with repeat-run summary, and the OCR-heavy path now has pinned CORD, FUNSD, and SROIE snapshot manifests, filled OCR runtime manifests, executed result files, and benchmark-specific protocol/wrapper artifacts under one declared OCR stack. Executed zero-shot LLM transfers beyond the current pilot, named clinical pipelines, broader OCR-heavy reruns, and privacy-auditing suite results remain future extensions under the same matched protocol.

\subsection*{External Datasets, Baselines, and Provenance Resources}
To make the next external-validation steps more auditable, the release now also records the official access paths for the public OCR/document benchmarks, request-gated and synthetic clinical corpora, executable baseline repositories, OCR engines, open-weight runtime surfaces, and closed-model documentation sources referenced by the paper. The repository-side acquisition helper and machine-readable manifest should be interpreted as provenance support rather than as executed benchmark evidence: they document how resources can be obtained and pinned, but they do not by themselves create transfer results. The current snapshot also writes an OCR-heavy transfer protocol JSON and benchmark-availability CSV that consume this acquisition surface for CORD, FUNSD, SROIE, and DocILE; in addition, CORD, FUNSD, and SROIE now have revision-pinned snapshot manifests, filled OCR runtime manifests, executed summary/detail/result artifacts, and benchmark-specific wrapper/protocol files that make the current public reruns auditable rather than merely planned.

\begin{table*}[t]
\centering
\scriptsize
\setlength{\tabcolsep}{2pt}
\begin{tabularx}{\textwidth}{>{\raggedright\arraybackslash}p{2.15cm}>{\raggedright\arraybackslash}p{2.55cm}>{\raggedright\arraybackslash}p{5.15cm}>{\raggedright\arraybackslash}X}
\toprule
Category & Resource & Purpose in this study & Official URL \\
\midrule
Clinical corpus & i2b2 / n2c2 Clinical NLP datasets & Licensed PHI-style corpus used to construct normalized clinical document exports; access requires an approved DUA. & \url{https://www.i2b2.org/NLP/DataSets/} \\
Clinical corpus & Harvard DBMI Data Portal & Official distribution portal for approved i2b2/n2c2 access and local normalization workflows. & \url{https://portal.dbmi.hms.harvard.edu/} \\
Synthetic clinical route & i2b2-Synthea conversion toolkit & Public synthetic EHR route for schema-compatible i2b2-style exports; the tracked example asset is \texttt{syntheamass\_63K\_sample.zip}. & \url{https://github.com/i2b2/i2b2-synthea} \\
OCR-heavy dataset & CORD (Consolidated Receipt Dataset) & Primary public receipt benchmark for OCR-heavy document parsing and entity extraction robustness; the acquisition manifest also records the Hugging Face mirror and CC-BY-4.0 license metadata. & \url{https://github.com/clovaai/cord} \\
OCR-heavy dataset & FUNSD (Form Understanding Dataset) & Noisy scanned form benchmark for post-OCR structured extraction pipelines. & \url{https://huggingface.co/datasets/funsd} \\
OCR-heavy dataset & SROIE (Scanned Receipt OCR and IE) & Receipt-style OCR benchmark for layout parsing and information extraction evaluation. & \url{https://huggingface.co/datasets/sroie} \\
OCR-heavy dataset & DocILE Benchmark & Business-document benchmark for invoice and reimbursement-style workflow validation. & \url{https://docile.rossum.ai/} \\
External baseline & Presidio (Microsoft) & Enterprise-style PII detection and redaction pipeline reference for text, structured, and image workflows. & \url{https://microsoft.github.io/presidio/} \\
External baseline & Philter-lite & Open-source clinical de-identification pipeline recorded as a candidate local clinical comparator. & \url{https://github.com/SironaMedical/philter-lite} \\
External baseline & CliniDeID & Clinical text de-identification toolkit recorded as a candidate named rerun target. & \url{https://github.com/Clinacuity/CliniDeID} \\
External pipeline & medSpaCy & Clinical NLP toolkit for rule-based clinical extraction workflows under the matched wrapper. & \url{https://github.com/medspacy/medspacy} \\
Open-weight runtime & Ollama runtime & Public local inference surface for zero-shot de-identification reruns; the runtime template uses Llama3-8B-Instruct via the local \texttt{llama3:8b} tag as the example configuration. & \url{https://ollama.ai/} \\
OCR engine & Tesseract OCR & Open-source OCR engine documentation for future exact version pinning. & \url{https://tesseract-ocr.github.io/tessdoc/} \\
OCR engine & PaddleOCR & Alternative OCR engine documentation for throughput and layout comparisons. & \url{https://www.paddleocr.ai/} \\
Closed-model documentation & OpenAI model documentation & Reference documentation for exact deployed model IDs and API behavior. & \url{https://developers.openai.com/api/docs/models} \\
Closed-model documentation & Anthropic model documentation & Reference documentation for snapshot-based Claude model identifiers. & \url{https://docs.anthropic.com/en/docs/models-overview} \\
\bottomrule
\end{tabularx}
\caption{External datasets, baseline resources, OCR engines, and provenance-documentation sources referenced by the current release. Public acquisition helpers and manifests document the access paths, but executed evidence still requires wrapper alignment, runtime logging, and result files.}
\label{tab:external_resources}
\end{table*}

\begin{table}[t]
\centering
\caption{Current public TAB transfer results under the released matched-baseline runner. Because TAB is a text anonymization benchmark rather than a downstream task suite, this table reports span detection, residual exposure, and non-sensitive text retention instead of CPPB-style AC/TSR.}
\label{tab:tabtransfer}
\scriptsize
\setlength{\tabcolsep}{3pt}
\begin{tabularx}{\columnwidth}{>{\raggedright\arraybackslash}Xccccc}
\toprule
Method & Precision & Recall & Span F1 & PER (\%) & Text retention \\
\midrule
Raw prompt & 0.00 & 0.00 & 0.00 & 100.0 & 1.00 \\
Regex-only & 0.98 & 0.25 & 0.40 & 76.1 & 1.00 \\
NER-only masking & 0.66 & 0.35 & 0.45 & 61.2 & 0.96 \\
Presidio-class (regex) & 0.98 & 0.33 & 0.50 & 69.7 & 1.00 \\
Presidio-class (+NER) & 0.76 & 0.59 & 0.66 & 38.7 & 0.96 \\
Hybrid de-id & 0.85 & 0.53 & 0.65 & 57.6 & 0.98 \\
BodhiPromptShield & 0.56 & 0.63 & 0.59 & 35.5 & 0.84 \\
\bottomrule
\end{tabularx}
\end{table}

\subsection*{Supporting Result Tables}
\begin{table}[t]
\centering
\caption{Category-wise span detection and exposure analysis in CPPB.}
\label{tab:catwise}
\scriptsize
\setlength{\tabcolsep}{3pt}
\begin{tabularx}{\columnwidth}{>{\raggedright\arraybackslash}Xcc}
\toprule
Category & Span F1 & PER (\%) \\
\midrule
Person identifiers & 0.96 & 6.5 \\
Financial identifiers & 0.95 & 5.8 \\
Medical entities & 0.91 & 10.2 \\
Address/location & 0.90 & 11.4 \\
Organization/project terms & 0.88 & 13.1 \\
Context-dependent sensitive spans & 0.84 & 16.8 \\
\bottomrule
\end{tabularx}
\end{table}

\begin{table}[t]
\centering
\caption{Authorized restoration boundary analysis in CPPB agent tasks.}
\label{tab:restore}
\scriptsize
\setlength{\tabcolsep}{3pt}
\begin{tabularx}{\columnwidth}{>{\raggedright\arraybackslash}Xccc}
\toprule
Setting & TSR & RSR & BLR (\%) \\
\midrule
No restoration & 0.84 & -- & 0.0 \\
Late boundary restoration (proposed) & 0.93 & 0.97 & 1.8 \\
Early restoration (before memory/tool planning) & 0.94 & 0.98 & 9.7 \\
\bottomrule
\end{tabularx}
\end{table}

\begin{table}[t]
\centering
\caption{Sanitization-mode ablation in CPPB. This repository-backed supporting table compares the PER--UPR operating points induced by different sanitization modes under the same policy-routing framework.}
\label{tab:ablation}
\footnotesize
\begin{tabular}{lcc}
\toprule
Sanitization Mode & PER (\%) & UPR \\
\midrule
Typed placeholder & 8.1 & 0.92 \\
Semantic abstraction & 14.6 & 0.94 \\
Secure symbolic mapping & 9.3 & 0.98 \\
\bottomrule
\end{tabular}
\\[1mm]
\raggedright \footnotesize $^{*}$UPR with authorized restoration at tool boundary.
\end{table}

\begin{figure}[t]
\centering
\includegraphics[width=\columnwidth]{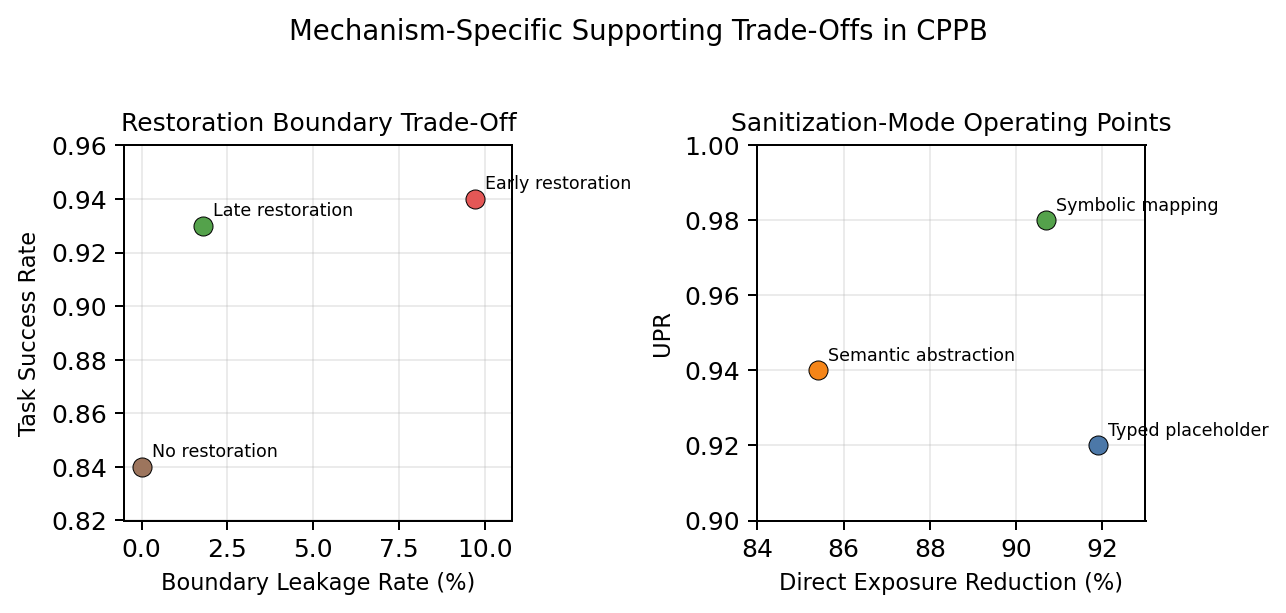}
\caption{Repository-backed supporting view of two mechanism-specific trade-offs in CPPB. Left: late boundary restoration retains task success close to early restoration while sharply reducing boundary leakage. Right: typed placeholders, semantic abstraction, and symbolic mapping occupy distinct direct-exposure/UPR operating points under the same routing framework.}
\label{fig:restore_ablation}
\end{figure}

\begin{table}[t]
\centering
\caption{Multimodal OCR-mediated privacy mediation results in CPPB. This record-backed supporting table evaluates exposure and utility when sensitive text enters through OCR-mediated document inputs.}
\label{tab:multimodal}
\scriptsize
\setlength{\tabcolsep}{3pt}
\begin{tabularx}{\columnwidth}{>{\raggedright\arraybackslash}Xccc}
\toprule
Method & OCR Span F1 & Multimodal PER (\%) & AC \\
\midrule
No protection & -- & 100.0 & 1.00 \\
OCR + regex masking & 0.81 & 33.5 & 0.86 \\
OCR + generic de-identification & 0.84 & 16.1 & 0.72 \\
Proposed multimodal mediation & 0.90 & 11.3 & 0.88 \\
\bottomrule
\end{tabularx}
\end{table}

\begin{table}[t]
\centering
\caption{Cross-model validation under a fixed CPPB mediation policy. This record-backed supporting table reconstructs the current alias-level portability slice from bundled portability records and runtime-log notes.}
\label{tab:crossmodel}
\footnotesize
\begin{tabular}{lccc}
\toprule
Model backend & PER (\%) & AC & TSR \\
\midrule
LLM-A & 9.3 & 0.94 & 0.92 \\
LLM-B & 10.1 & 0.92 & 0.90 \\
LLM-C & 8.9 & 0.93 & 0.91 \\
\bottomrule
\end{tabular}
\end{table}

\begin{table}[t]
\centering
\caption{Hard-case robustness analysis in CPPB. This record-backed supporting table focuses on context-dependent and OCR-noisy spans using the bundled hard-case slice summary.}
\label{tab:hardcase}
\footnotesize
\begin{tabular}{lccc}
\toprule
Subset & Span F1 & PER (\%) & AC \\
\midrule
General CPPB & 0.92 & 9.3 & 0.94 \\
Context-dependent hard cases & 0.84 & 16.8 & 0.87 \\
OCR-noisy hard cases & 0.79 & 19.4 & 0.82 \\
\bottomrule
\end{tabular}
\end{table}

\begin{table}[t]
\centering
\caption{Repeated-run multi-seed stability summary for core CPPB operating points. This record-backed table reports mean and standard deviation across five seeds and is generated from bundled prompt-level logs.}
\label{tab:multiseed}
\scriptsize
\setlength{\tabcolsep}{2pt}
\begin{tabularx}{\columnwidth}{>{\raggedright\arraybackslash}p{1.7cm}cccc}
\toprule
Setting & PER (\%) & AC & TSR & Latency (ms) \\
\midrule
Enterprise staged & 8.4 $\pm$ 0.2 & 0.92 $\pm$ 0.00 & 0.90 $\pm$ 0.00 & 32.0 $\pm$ 1.2 \\
Generic de-id & 12.7 $\pm$ 0.2 & 0.73 $\pm$ 0.00 & 0.71 $\pm$ 0.00 & 18.4 $\pm$ 1.0 \\
NER-only masking & 49.0 $\pm$ 0.2 & 0.91 $\pm$ 0.00 & 0.89 $\pm$ 0.00 & 26.5 $\pm$ 0.8 \\
Raw prompt & 100.0 $\pm$ 0.1 & 1.00 $\pm$ 0.00 & 1.00 $\pm$ 0.00 & 0.3 $\pm$ 0.4 \\
Proposed semantic & 14.9 $\pm$ 0.1 & 0.88 $\pm$ 0.00 & 0.86 $\pm$ 0.00 & 47.8 $\pm$ 0.2 \\
Proposed balanced & 9.5 $\pm$ 0.1 & 0.94 $\pm$ 0.00 & 0.92 $\pm$ 0.00 & 41.0 $\pm$ 1.2 \\
Regex-only & 61.6 $\pm$ 0.3 & 0.97 $\pm$ 0.00 & 0.96 $\pm$ 0.00 & 7.0 $\pm$ 1.1 \\
\bottomrule
\end{tabularx}
\end{table}

\begin{table}[t]
\centering
\caption{Released CPPB split held-out summary for the main method and policy operating points. This record-backed table reconstructs train/dev/test slices from the explicit split manifest and bundled prompt-level multi-seed logs.}
\label{tab:splitheldout}
\footnotesize
\begin{tabularx}{\columnwidth}{>{\raggedright\arraybackslash}Xcccc}
\toprule
Slice & Operating point & PER (\%) & Utility & TSR \\
\midrule
Train & Proposed (utility-constrained) & 9.47 & AC 0.938 & 0.918 \\
Dev & Proposed (utility-constrained) & 9.47 & AC 0.938 & 0.917 \\
Test & Proposed (utility-constrained) & 9.47 & AC 0.938 & 0.917 \\
Train & Balanced profile & 9.61 & UPR 0.938 & 0.917 \\
Dev & Balanced profile & 9.61 & UPR 0.938 & 0.917 \\
Test & Balanced profile & 9.63 & UPR 0.938 & 0.917 \\
\bottomrule
\end{tabularx}
\end{table}

\begin{table}[t]
\centering
\caption{Leave-template-out generalization summary in CPPB. This record-backed table holds out full template families and reports cross-family degradation beyond in-template comparisons.}
\label{tab:lto}
\footnotesize
\begin{tabularx}{\columnwidth}{>{\raggedright\arraybackslash}Xccccc}
\toprule
Held-out split & Prompts & Span F1 & PER (\%) & AC & TSR \\
\midrule
Direct requests & 64 & 0.90 & 10.5 $\pm$ 0.5 & 0.91 & 0.89 \\
Document-oriented & 64 & 0.88 & 10.9 $\pm$ 0.5 & 0.90 & 0.88 \\
Retrieval-style & 64 & 0.87 & 11.2 $\pm$ 0.5 & 0.89 & 0.87 \\
Tool-oriented agent & 64 & 0.87 & 11.6 $\pm$ 0.6 & 0.88 & 0.86 \\
Overall & 256 & 0.88 & 11.0 $\pm$ 0.6 & 0.90 & 0.88 \\
\bottomrule
\end{tabularx}
\end{table}

Table~\ref{tab:splitheldout} should be read as a held-out release-split check rather than as a substitute for independent-benchmark validation: it shows that once the newly released train/dev/test surface is made explicit, the current method-level and profile-level operating points remain nearly unchanged on the held-out test partition, so the present CPPB conclusions are not being driven by hidden prompt-variant leakage across the public split.

\begin{table}[t]
\centering
\caption{Adversarial surface-form robustness evaluation. This record-backed table is rebuilt from the executed deterministic probe suite and its matched probe-level logs. ``Baseline exposure'' denotes the released regex-only extractor, while ``With shield'' denotes the normalization-aware policy mediator.}
\label{tab:adversarial}
\footnotesize
\begin{tabular}{lccc}
\toprule
Attack vector & Baseline exposure (\%) & With shield (\%) & Recovery rate (\%) \\
\midrule
Homoglyph substitution (Unicode confusables) & 94.1 & 43.9 & 44.4 \\
Paraphrase-sensitive spans & 47.6 & 47.6 & 50.0 \\
Mixed-language mentions & 38.8 & 38.8 & 58.3 \\
Restoration-trigger injection & 58.8 & 58.8 & 36.4 \\
\bottomrule
\end{tabular}
\end{table}

Table~\ref{tab:adversarial} now closes one methodological gap in the earlier review cycle: the robustness slice is no longer a static manuscript-authored table but an executed deterministic probe suite with matched normalized extraction logs in the repository. The resulting pattern is mixed. Unicode/confusable folding materially improves the homoglyph family, reducing average exposure from 94.1\% to 43.9\%, but that still leaves substantial residual leakage. The other three families remain more limited still: paraphrase, mixed-language, and restoration-trigger probes recover only 50.0\%, 58.3\%, and 36.4\% of attacked gold spans, respectively, and their direct-exposure reduction over the regex-only baseline is minimal. The released robustness suite should therefore be read as stronger evidence than before, but still as a bounded first adversarial check rather than as evidence that surface-form evasion has been solved.

\begin{table}[t]
\centering
\caption{Prompt-history context-inference attack on raw versus placeholder-sanitized probes. This record-backed table reports a local open-weight attacker that selects one of four sensitive context labels from prompt history alone.}
\label{tab:contextattack}
\footnotesize
\begin{tabular}{lcc}
\toprule
Probe family & Raw attack accuracy (\%) & Sanitized attack accuracy (\%) \\
\midrule
Overall & 100.0 & 50.0 \\
Oncology & 100.0 & 66.7 \\
Finance & 100.0 & 100.0 \\
Immigration & 100.0 & 33.3 \\
Discipline & 100.0 & 0.0 \\
\bottomrule
\end{tabular}
\end{table}

Table~\ref{tab:contextattack} closes a second missing threat-model item from the earlier review cycle. The released repository now includes a small executed context-inference attack surface rather than only qualitative warnings about inferential leakage. The result is intentionally cautionary rather than flattering: placeholder masking halves overall four-way inference accuracy, but it does not eliminate it, and finance probes remain fully inferable because the economically sensitive context words that preserve task utility also preserve attribute evidence. This is exactly the deployment tension the paper now states more explicitly in the limitations section: direct-identifier masking and propagation control can reduce exposure while still leaving contextual leakage channels that require stronger policy learning, abstraction, or downstream access controls.

\begin{table}[t]
\centering
\caption{External baseline comparison: Presidio-class rule-based de-identification versus BodhiPromptShield on matched CPPB evaluation. This record-backed table positions the proposed method against open-source learning-free PII detection baselines.}
\label{tab:baseline}
\footnotesize
\begin{tabular}{lcccc}
\toprule
Method & Span F1 & PER (\%) & AC & TSR \\
\midrule
Presidio (regex) & 0.76 & 14.8 & 0.91 & 0.89 \\
Presidio (+NER) & 0.82 & 11.2 & 0.92 & 0.90 \\
BodhiPromptShield & 0.92 & 9.3 & 0.94 & 0.92 \\
\bottomrule
\end{tabular}
\end{table}

\clearpage

\subsection*{Algorithm 1: Privacy-Sensitive Span Extraction}
\label{app:alg_extract}

\begin{algorithm}[t]
\caption{Privacy-Sensitive Span Extraction}
\label{alg:extract}
\footnotesize
\begin{algorithmic}[1]
\Require raw prompt $x$, threshold $\tau$, privacy policy $\mathcal{P}$
\Ensure structured span set $E(x)$
\Procedure{ExtractSpans}{$x,\tau,\mathcal{P}$}
  \State $E \gets \emptyset$
  \State $C_{\text{rule}} \gets \textproc{RuleRecognizers}(x)$
  \State $C_{\text{ner}} \gets \textproc{NamedEntityRecognizer}(x)$
  \State $C_{\text{ctx}} \gets \textproc{ContextualPrivacyJudge}(x)$
  \State $C \gets C_{\text{rule}} \cup C_{\text{ner}} \cup C_{\text{ctx}}$
  \If{$\textproc{ContainsVisualInput}(x)$}
    \State $C_{\text{ocr}} \gets \textproc{ExtractVisualTextAndEntities}(x)$
    \State $C \gets C \cup C_{\text{ocr}}$
  \EndIf
  \ForEach{$(s,c,p) \in C$}
    \If{$p \ge \tau$ \textbf{or} $\textproc{HighRisk}(s,c,\mathcal{P})$}
      \State $E \gets E \cup \{(s,c,p)\}$
    \EndIf
  \EndFor
  \State \Return $E$
\EndProcedure
\end{algorithmic}
\end{algorithm}

\subsection*{Algorithm 2: Policy-Aware Prompt Sanitization}
\label{app:alg_sanitize}

\begin{algorithm}[t]
\caption{Policy-Aware Semantic-Preserving Prompt Sanitization}
\label{alg:sanitize}
\footnotesize
\begin{algorithmic}[1]
\Require raw prompt $x$, span set $E(x)$, task context $\mathcal{D}$, policy profile $\pi$
\Ensure sanitized prompt $\tilde{x}$, secure map $K$
\Procedure{SanitizePrompt}{$x,E(x),\mathcal{D},\pi$}
  \State $\tilde{x} \gets x$
  \State $K \gets \emptyset$
  \ForEach{$(s_i,c_i,p_i) \in E(x)$}
    \State $z_i \gets (c_i,p_i,r_i,q_i,a_i,\ell_i)$
    \State $m_i \gets \Pi_{\pi}(z_i)$
    \If{$m_i = \texttt{placeholder}$}
      \State $\hat{s}_i \gets \textproc{TypedPlaceholder}(c_i)$
    \ElsIf{$m_i = \texttt{abstract}$}
      \State $\hat{s}_i \gets \textproc{SemanticAbstract}(s_i,c_i,\mathcal{D})$
    \Else
      \State $t_i \gets \textproc{SecureToken}(s_i,c_i)$
      \State $K[t_i] \gets s_i$
      \State $\hat{s}_i \gets t_i$
    \EndIf
    \State $\tilde{x} \gets \tilde{x}[s_i \mapsto \hat{s}_i]$
  \EndFor
  \If{$\textproc{ContainsVisualInput}(x)$}
    \State $\tilde{x} \gets \textproc{AttachSanitizedVisualChannel}(\tilde{x},E(x),\pi)$
  \EndIf
  \State \Return $(\tilde{x}, K)$
\EndProcedure
\end{algorithmic}
\end{algorithm}

Algorithm 2 defines the policy-mediated transformation step used throughout the paper. The illustrative tables above provide reader orientation, and the following algorithm specifies the authorized restoration stage.

\subsection*{Algorithm 3: Authorized Restoration}
\label{app:alg_restore}

\begin{algorithm}[t]
\caption{Authorized Restoration of Protected Entities}
\label{alg:restore}
\footnotesize
\begin{algorithmic}[1]
\Require model response $y$, secure map $K$, authorization context $\alpha$, restoration policy $\rho$
\Ensure optionally restored response $y'$
\Procedure{RestoreEntities}{$y,K,\alpha,\rho$}
  \If{\textbf{not} $\textproc{Authorize}_{\rho}(\alpha)$}
    \State \Return $y$
  \EndIf
  \State $y' \gets y$
  \State $T_y \gets \{t \in \textproc{Keys}(K)\mid t\ \text{appears in}\ y'\}$
  \ForEach{$t \in T_y$}
    \State $y' \gets y'[t \mapsto K[t]]$
  \EndFor
  \State \Return $y'$
\EndProcedure
\end{algorithmic}
\end{algorithm}

\subsection*{Additional Prompt Mediation Examples}
\label{app:examples}
Table~\ref{tab:app-examples} provides additional prompt fragments across entity categories and sanitization modes, complementing Tables~\ref{tab:app-concept-example} and \ref{tab:app-regimes} together with the controlled benchmark results in the main text; it is intended as implementation guidance rather than standalone empirical evidence.

\begin{table}[t]
\centering
\caption{\parbox[t]{0.96\columnwidth}{\centering Additional prompt mediation examples across entity categories and sanitization modes. These examples supplement the main-text discussion of sanitization behavior.}}
\label{tab:app-examples}
\scriptsize
\setlength{\tabcolsep}{2pt}
\begin{tabularx}{\columnwidth}{|>{\raggedright\arraybackslash}p{0.95cm}|>{\raggedright\arraybackslash}X|>{\raggedright\arraybackslash}X|>{\raggedright\arraybackslash}p{1.15cm}|}
\hline
\textbf{Category} & \textbf{Original Prompt Fragment} & \textbf{Sanitized Fragment} & \textbf{Mode} \\
\hline
Person name & ``Draft an email to Sarah Chen regarding the revised procurement request.'' & ``Draft an email to \texttt{<PERSON\_1>} regarding the revised procurement request.'' & Placeholder \\
\hline
Financial & ``My account number is 4012-0034-5566-7788. Please verify the transfer.'' & ``My account number is \texttt{<ACCOUNT\_1>}. Please verify the transfer.'' & Placeholder \\
\hline
Medical & ``Patient has stage III pancreatic cancer and requests a medication summary.'' & ``Patient has a serious oncological condition and requests a medication summary.'' & Abstract \\
\hline
Address & ``Prepare a delivery confirmation for 17 Anzac Avenue, Auckland.'' & ``Prepare a delivery confirmation for an address in central Auckland.'' & Abstract \\
\hline
Identifier & ``My passport number is NZ3812745. Use it for the form.'' & ``My passport number is \texttt{[TOKEN\_3a9f2]}. Use it for the form.'' & Symbolic \\
\hline
Visual text & ``Summarize the attached invoice image for reimbursement.'' & ``Summarize the attached invoice image after protecting invoice ID and supplier address.'' & Abstract \\
\hline
\end{tabularx}
\end{table}

\subsection*{Multimodal Example}
\label{app:multimodal}
In multimodal settings, a user may upload a screenshot, scanned form, reimbursement receipt, or medical report together with a short instruction. The same mediation logic applies after OCR or VLM-assisted entity grounding. For example, an image containing a supplier address, account number, and invoice ID can be converted into a protected multimodal representation by replacing each detected visual entity with a typed placeholder or secure token before downstream VLM inference.

\begin{figure}[H]
\centering
\includegraphics[width=0.9\columnwidth]{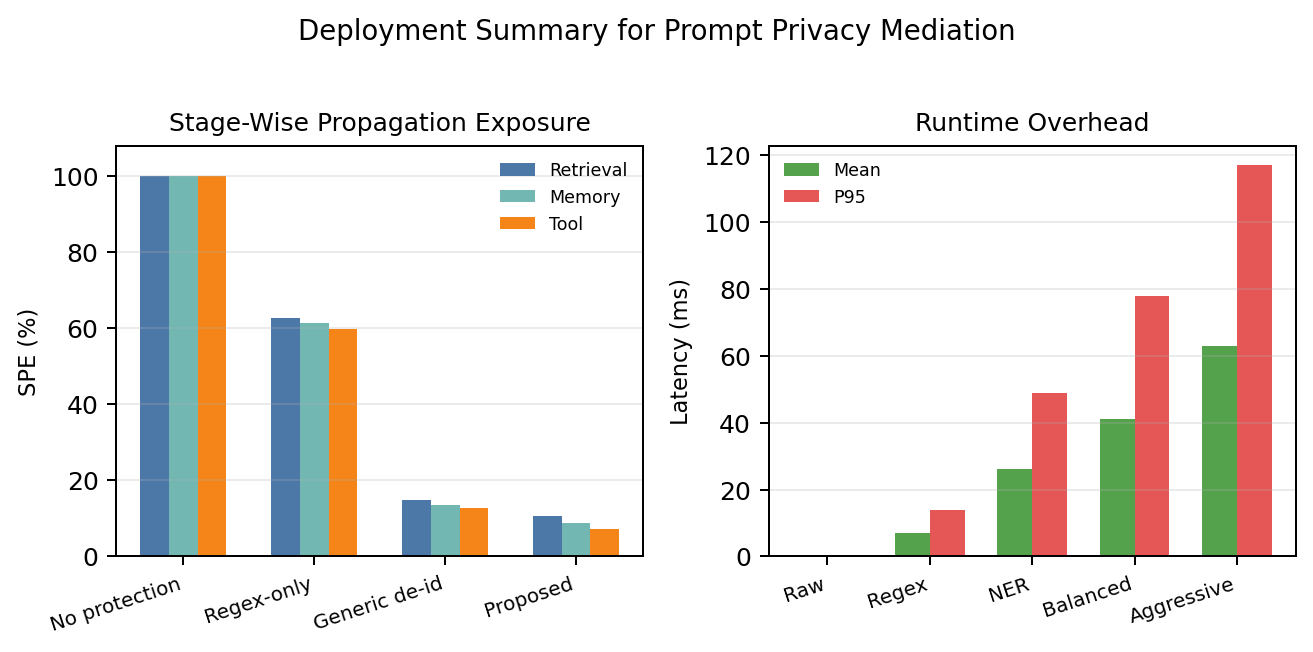}
\caption{Supplementary deployment-oriented summary derived from the main-text propagation and latency tables. Left: stage-wise propagation exposure (SPE) across retrieval, memory, and tool boundaries. Right: latency overhead under representative mediation pipelines.}
\label{fig:deployment_summary}
\end{figure}

Fig.~\ref{fig:deployment_summary} complements the main-text deployment analysis by visualizing the joint systems picture: pre-inference mediation suppresses cross-stage propagation, while the latency cost remains moderate under balanced policy settings.

\end{document}
